# Supplementary material for: Nozzle Shocks, Disk Tearing and Streamers Drive Rapid Accretion in 3D GRMHD Simulations of Warped Thin Disks
Source: arXiv:2210.10053 source file (2024-05-06)
Supplement: Supplementary file 1 [file appendix.tex]

\appendix
